# Supplementary material for: Proteins with greater influence on network dynamics evolve more slowly but are not more essential
Source: arXiv:0909.2889 source file (2009-09-20)
Supplement: Supplementary file 1 [file SupplementaryText.pdf]

# Proteins with greater influence on network dynamics evolve slower but are not more essential

## Supporting data

Ryan N. Gutenkunst
(Dated: September 15, 2009)

## I. FOCUS ON "OUTPUT" VARIABLES

| system | $r_{dN/dS,D}$ (p-val, N) | "output" variables |
|---|---|---|
| Insulin/EGF signaling [1] | -0.24 (0.23, 12) | active ERK |
| Heregulin/EGF signaling [2] | -0.33 (0.16, 12) | active ERK and active Akt |
| NGF/EGF signaling (smaller) [3] | -0.73 (0.03, 8) | active ERK |
| NGF/EGF signaling (larger) [4] | -0.40 (0.05, 16) | active ERK |
| EGF receptor endocytosis [5] | -0.19 (0.21, 24) | active ERK |
| Wnt/ERK crosstalk [6] | -0.02 (0.54, 10) | $\beta$-catenin/TCF complex |
| IL6 signaling [7] | -0.05 (0.69, 9) | nuclear STAT3 |
| G1 cell cycle progression [8] | -0.57 (0.05, 9) | hypo- and hyper-phosphorylated Rb |
| Rho-kinase activation [9] | -0.19 (0.28, 15) | phosphorylated myosin light chain |
| Arachidonic acid metabolism [10] | -0.57 (0.05, 10) | PGE2 and LTB4 |
| TNF-driven apoptosis [11] | -0.22 (0.34, 12) | the apoptosome |
| $\beta$-adrenergic signaling [12] | -0.18 (0.32, 9) | active MAP kinase |
| expected sign | − | |
| total of expected sign | 12 | |

TABLE I: Correlations when $D$ calculated using "output" variables only.

In an attempt to be agnostic about which molecular species are truly important for fitness, the measure of dynamical influence $D$ reported in the main text considers effects on the dynamics of *all* molecular species in the system. However, in many systems one or a few molecular species are considered "outputs". It might be expected that these variables are more important for fitness than are the internal variables. To assess this, for each system studied we measured $\kappa$ using only variables deemed "output" in the original publications. Table I reports the resulting correlations and the variables which were considered outputs. Figure 1 plots the resulting correlations. In these analyses, the variables considered output are not themselves included, as they will trivially have large $D$.

With $D$ calculated considering only output variables, all 12 systems show a negative correlation between dN/dS and $D$. The correlations are, however, not consistently stronger than those when $D$ was calculated including all variables, and they are often dominated by a single outlier point with high $D$. This may suggest that many of the "internal" variables effect fitness through more than just the "output" variables. This is perhaps unsurprising given the ubiquity of cross-talk in biochemical networks.

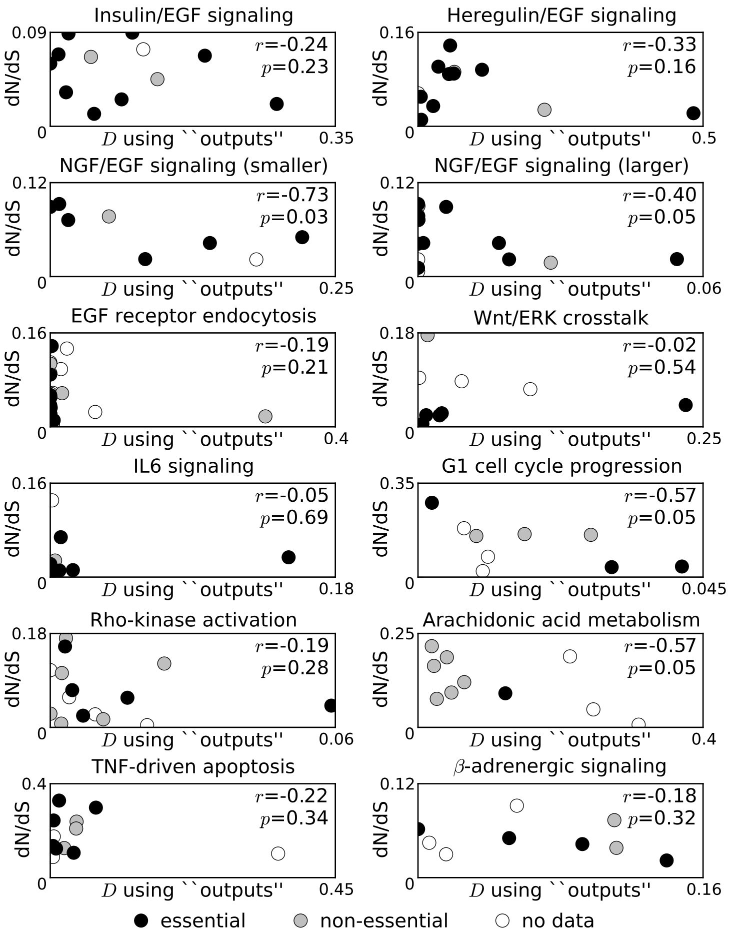


FIG. 1: $D$ calculated using only “output” variables.

## II. USING ONLY MAMMALIAN SEQUENCES

| system | $r_{dN/dS,D}$ (p-val, N) |
|---|---|
| Insulin/EGF signaling [1] | -0.28 (0.17, 13) |
| Heregulin/EGF signaling [2] | -0.23 (0.21, 14) |
| NGF/EGF signaling (smaller) [3] | -0.58 (0.07, 8) |
| NGF/EGF signaling (larger) [4] | -0.27 (0.15, 17) |
| EGF receptor endocytosis [5] | -0.03 (0.45, 25) |
| Wnt/ERK crosstalk [6] | -0.37 (0.14, 10) |
| IL6 signaling [7] | -0.30 (0.21, 10) |
| G1 cell cycle progression [8] | -0.31 (0.19, 10) |
| Rho-kinase activation [9] | -0.10 (0.40, 16) |
| Arachidonic acid metabolism [10] | -0.49 (0.08, 10) |
| TNF-driven apoptosis [11] | -0.11 (0.41, 12) |
| $\beta$-adrenergic signaling [12] | +0.70 (0.98, 9) |
| expected sign | − |
| total of expected sign | 11 |

TABLE II: dN/dS using only mammalian sequences.

Table II reports correlations between $D$ and dN/dS using only sequences from mammals. The resulting correlations are all of the same sign as when all chicken and zebrafish are included, although they are typically slightly weaker.

## III. EXCLUDING SHARED PROTEINS

| system | $r_{dN/dS,D}$ (p-val, N) |
|---|---|
| Insulin/EGF signaling [1] | -0.61 (0.08, 6) |
| Heregulin/EGF signaling [2] | -0.63 (0.06, 6) |
| NGF/EGF signaling (smaller) [3] | — (—, 1) |
| NGF/EGF signaling (larger) [4] | -0.39 (0.21, 7) |
| EGF receptor endocytosis [5] | -0.01 (0.49, 10) |
| Wnt/ERK crosstalk [6] | -0.42 (0.16, 7) |
| IL6 signaling [7] | -0.28 (0.24, 10) |
| G1 cell cycle progression [8] | -0.31 (0.19, 10) |
| Rho-kinase activation [9] | -0.26 (0.20, 14) |
| Arachidonic acid metabolism [10] | -0.53 (0.06, 10) |
| TNF-driven apoptosis [11] | -0.14 (0.36, 12) |
| $\beta$-adrenergic signaling [12] | +0.26 (0.71, 7) |
| expected sign | − |
| total of expected sign | 10 |

TABLE III: Correlations with shared proteins removed.

Several of the systems we consider share proteins between them, so they are not independent assessments of the relationship between $D$ and dN/dS. To make them independent, Table III reports correlations when all proteins shared between two or more systems are ignored. In this analysis, the smaller NGF/EGF signaling model cannot be used, because it contains only a single unique protein. Similar to our previous analysis, all systems save the $\beta$-adrenergic signaling system yield a negative correlation.

| system | $r_{dN,D}$ (p-val, N) | $r_{dS,D}$ (p-val, N) |
|---|---|---|
| Insulin/EGF signaling [1] | -0.29 (0.17, 13) | -0.40 (0.09, 13) |
| Heregulin/EGF signaling [2] | -0.25 (0.20, 14) | -0.30 (0.15, 14) |
| NGF/EGF signaling (smaller) [3] | -0.65 (0.03, 8) | -0.46 (0.11, 8) |
| NGF/EGF signaling (larger) [4] | -0.41 (0.03, 17) | -0.01 (0.46, 17) |
| EGF receptor endocytosis [5] | -0.07 (0.39, 25) | -0.16 (0.22, 25) |
| Wnt/ERK crosstalk [6] | -0.34 (0.16, 10) | +0.29 (0.79, 10) |
| IL6 signaling [7] | -0.04 (0.50, 9) | +0.04 (0.55, 9) |
| G1 cell cycle progression [8] | -0.41 (0.13, 9) | -0.22 (0.30, 9) |
| Rho-kinase activation [9] | -0.32 (0.09, 15) | +0.36 (0.93, 15) |
| Arachidonic acid metabolism [10] | -0.17 (0.32, 10) | +0.56 (0.92, 10) |
| TNF-driven apoptosis [11] | +0.21 (0.74, 11) | -0.33 (0.15, 11) |
| $\beta$-adrenergic signaling [12] | +0.35 (0.80, 8) | +0.07 (0.56, 8) |
| expected sign | − | − |
| total of expected sign | 10 | 7 |

TABLE IV: Correlations of dynamical influence $D$ with dN and dS.

## IV. dS AND dN CONSIDERED SEPARATELY

Table IV reports the correlation between dynamical influence $D$ and dN and dS. Here dN and dS were calculated using human and mouse sequences. The correlation between $D$ and dS is inconsistent in sign, suggesting that the negative correlations we see with dN/dS do not simply reflect correlation with mutation rate (dS).

## V. GENE COMPACTNESS

| system | $r_{dN/dS,C}$ (p-val, N) | $r_{D,C}$ (p-val, N) | $r_{dN/dS,D\|C}$ |
|---|---|---|---|
| Insulin/EGF signaling [1] | +0.11 (0.62, 11) | +0.50 (0.94, 11) | -0.49 |
| Heregulin/EGF signaling [2] | +0.20 (0.75, 14) | +0.01 (0.53, 14) | -0.27 |
| NGF/EGF signaling (smaller) [3] | +0.29 (0.74, 7) | -0.39 (0.20, 7) | -0.59 |
| NGF/EGF signaling (larger) [4] | +0.00 (0.52, 16) | -0.11 (0.38, 16) | -0.41 |
| EGF receptor endocytosis [5] | -0.01 (0.50, 25) | +0.39 (0.96, 25) | -0.11 |
| Wnt/ERK crosstalk [6] | +0.73 (0.99, 10) | -0.31 (0.19, 10) | -0.15 |
| IL6 signaling [7] | +0.07 (0.69, 10) | +0.63 (0.96, 10) | -0.41 |
| G1 cell cycle progression [8] | +0.41 (0.88, 10) | +0.25 (0.76, 10) | -0.46 |
| Rho-kinase activation [9] | +0.74 (1.00, 16) | -0.34 (0.06, 16) | +0.07 |
| Arachidonic acid metabolism [10] | -0.55 (0.06, 10) | +0.28 (0.81, 10) | -0.47 |
| TNF-driven apoptosis [11] | -0.44 (0.07, 12) | +0.04 (0.58, 12) | -0.14 |
| $\beta$-adrenergic signaling [12] | +0.22 (0.75, 10) | -0.41 (0.14, 10) | +0.54 |
| expected sign | + | − | − |
| total of expected sign | 9 | 5 | 10 |

TABLE V: Correlations with gene compactness $C$.

Recently, gene compactness (the ratio of translated to transcribed sequence) was found to correlate positively with evolutionary rate in mammals [13]. Here we define gene compactness as the ratio of coding sequence length to transcript length defined in Ensembl [14]. For genes with multiple recorded transcripts, the most compact was used. Results are shown in Table V. Compactness is positively correlated with evolutionary rate in 9 of our 12 systems. However, we observe no consistent correlation between compactness and dynamical influence. It is thus unsurprising that gene compactness and dynamical influence exert independent effects on evolutionary rate, as evidenced by the fact that partial correlation controlling for compactness only changes one $D$-dN/dS correlation sign.

## VI. NUMBER OF REACTIONS

| system | $r_{dN/dS,Nrxn}$ (p-val, N) | $r_{D,Nrxn}$ (p-val, N) | $r_{dN/dS,D\|Nrxn}$ |
|---|---|---|---|
| Insulin/EGF signaling [1] | +0.12 (0.65, 13) | +0.32 (0.86, 13) | -0.42 |
| Heregulin/EGF signaling [2] | +0.03 (0.55, 14) | -0.60 (0.01, 14) | -0.31 |
| NGF/EGF signaling (smaller) [3] | -0.16 (0.35, 8) | -0.40 (0.17, 8) | -0.79 |
| NGF/EGF signaling (larger) [4] | +0.05 (0.57, 17) | +0.23 (0.82, 17) | -0.45 |
| EGF receptor endocytosis [5] | -0.40 (0.02, 25) | -0.27 (0.09, 25) | -0.24 |
| Wnt/ERK crosstalk [6] | -0.43 (0.11, 10) | -0.47 (0.09, 10) | -0.66 |
| IL6 signaling [7] | -0.42 (0.03, 10) | +0.37 (0.82, 10) | -0.14 |
| G1 cell cycle progression [8] | -0.32 (0.20, 10) | -0.32 (0.18, 10) | -0.45 |
| Rho-kinase activation [9] | -0.02 (0.52, 16) | -0.26 (0.10, 16) | -0.22 |
| Arachidonic acid metabolism [10] | +0.03 (0.53, 10) | -0.26 (0.25, 10) | -0.54 |
| TNF-driven apoptosis [11] | — | — | — |
| $\beta$-adrenergic signaling [12] | +0.15 (0.68, 10) | -0.54 (0.05, 10) | +0.57 |
| expected sign | − | + | − |
| total of expected sign | 6 | 3 | 10 |

TABLE VI: Correlations with number of reactions $Nrxn$ involved in.

It might be expected that proteins involved in more reactions, i.e. with higher reaction degree, would have greater dynamical influence. As shown in Table VI, however, this is not the case. Moreover, proteins involved in more reactions do not evolve slower. It is thus clear that the correlation between dynamical influence and evolutionary rate is not explained by reaction degree. Note that in this analysis the TNF-driven apoptosis model could not be considered because it was not formulated in terms of discrete reactions.


[1] Borisov N, Aksamitiene E, Kiyatkin A, Legewie S, Berkhout J, et al. (2009) Systems-level interactions between insulin-EGF networks amplify mitogenic signaling. Mol Syst Biol 5: 256.

[2] Birtwistle MR, Hatakeyama M, Yumoto N, Ogunnaike BA, Hoek JB, et al. (2007) Ligand-dependent responses of the erbb signaling network: experimental and modeling analyses. Mol Syst Biol 3: 144.

[3] Brown KS, Hill CC, Calero GA, Myers CR, Lee KH, et al. (2004) The statistical mechanics of complex signaling networks: nerve growth factor signaling. Phys Biol 1: 184–195.

[4] Sasagawa S, Ozaki Y, Fujita K, Kuroda S (2005) Prediction and validation of the distinct dynamics of transient and sustained ERK activation. Nat Cell Biol 7: 365–373.

[5] Ung CY, Li H, Ma XH, Jia J, Li BW, et al. (2008) Simulation of the regulation of EGFR endocytosis and EGFR-ERK signaling by endophilin-mediated RhoA-EGFR crosstalk. FEBS Lett 582: 2283–2290.

[6] Kim D, Rath O, Kolch W, Cho KH (2007) A hidden oncogenic positive feedback loop caused by crosstalk between Wnt and ERK pathways. Oncogene 26: 4571–4579.

[7] Singh A, Jayaraman A, Hahn J (2006) Modeling regulatory mechanisms in IL-6 signal transduction in hepatocytes. Biotechnol Bioeng 95: 850–862.

[8] Haberichter T, Mdge B, Christopher RA, Yoshioka N, Dhiman A, et al. (2007) A systems biology dynamical model of mammalian G1 cell cycle progression. Mol Syst Biol 3: 84.

[9] Maeda A, Ozaki Y, Sivakumaran S, Akiyama T, Urakubo H, et al. (2006) $Ca^{2+}$-independent phospholipase A2-dependent sustained Rho-kinase activation exhibits all-or-none response. Genes Cells 11: 1071–1083.

[10] Yang K, Ma W, Liang H, Ouyang Q, Tang C, et al. (2007) Dynamic simulations on the arachidonic acid metabolic network. PLoS Comput Biol 3: e55.

[11] Albeck JG, Burke JM, Spencer SL, Lauffenburger DA, Sorger PK (2008) Modeling a snap-action, variable-delay switch controlling extrinsic cell death. PLoS Biol 6: e299.

[12] Neves SR, Tsokas P, Sarkar A, Grace EA, Rangamani P, et al. (2008) Cell shape and negative links in regulatory motifs together control spatial information flow in signaling networks. Cell 133: 666–680.

[13] Liao BY, Scott NM, Zhang J (2006) Impacts of gene essentiality, expression pattern, and gene compactness on the evolutionary rate of mammalian proteins. Mol Biol Evol 23: 2072–2080.

[14] Hubbard TJP, Aken BL, Beal K, Ballester B, Caccamo M, et al. (2006) Ensembl 2007. Nucl Acids Res 35: D610–617.
