# Supplementary material for: Proteins with greater influence on network dynamics evolve more slowly but are not more essential
Source: arXiv:0909.2889 source file (2009-09-20)
Supplement: Supplementary file 2 [file supp_dN_dS.tex]

\begin{tabular}{ccc}
system & $r_{dN,D}$ (p-val, N) & $r_{dS,D}$ (p-val, N)\\
\hline
Insulin/EGF signaling \cite{bib:Borisov2009} & -0.29 (0.17, 13) & -0.40 (0.09, 13)\\
Heregulin/EGF signaling \cite{bib:Birtwistle2007} & -0.25 (0.20, 14) & -0.30 (0.15, 14)\\
NGF/EGF signaling (smaller) \cite{bib:Brown2004} & -0.65 (0.03, 8) & -0.46 (0.11, 8)\\
NGF/EGF signaling (larger) \cite{bib:Sasagawa2005} & -0.41 (0.03, 17) & -0.01 (0.46, 17)\\
EGF receptor endocytosis \cite{bib:Ung2008} & -0.07 (0.39, 25) & -0.16 (0.22, 25)\\
Wnt/ERK crosstalk \cite{bib:Kim2007} & -0.34 (0.16, 10) & +0.29 (0.79, 10)\\
IL6 signaling \cite{bib:Singh2006} & -0.04 (0.50, 9) & +0.04 (0.55, 9)\\
G1 cell cycle progression \cite{bib:Haberichter2007} & -0.41 (0.13, 9) & -0.22 (0.30, 9)\\
Rho-kinase activation \cite{bib:Maeda2006} & -0.32 (0.09, 15) & +0.36 (0.93, 15)\\
Arachidonic acid metabolism \cite{bib:Yang2007} & -0.17 (0.32, 10) & +0.56 (0.92, 10)\\
TNF-driven apoptosis \cite{bib:Albeck2008} & +0.21 (0.74, 11) & -0.33 (0.15, 11)\\
$\beta$-adrenergic signaling \cite{bib:Neves2008} & +0.35 (0.80, 8) & +0.07 (0.56, 8)\\
\hline
expected sign & $-$ & $-$ \\
 total of expected sign & 10 & 7 \\
\end{tabular}
