# Supplementary material for: Proteins with greater influence on network dynamics evolve more slowly but are not more essential
Source: arXiv:0909.2889 source file (2009-09-20)
Supplement: Supplementary file 3 [file supp_important.tex]

\begin{tabular}{ccc}
system & $r_{dN/dS,D}$ (p-val, N) & ``output'' variables\\
\hline
Insulin/EGF signaling \cite{bib:Borisov2009} & -0.24 (0.23, 12) & active ERK\\
Heregulin/EGF signaling \cite{bib:Birtwistle2007} & -0.33 (0.16, 12) & active ERK and active Akt\\
NGF/EGF signaling (smaller) \cite{bib:Brown2004} & -0.73 (0.03, 8) & active ERK\\
NGF/EGF signaling (larger) \cite{bib:Sasagawa2005} & -0.40 (0.05, 16) & active ERK\\
EGF receptor endocytosis \cite{bib:Ung2008} & -0.19 (0.21, 24) & active ERK\\
Wnt/ERK crosstalk \cite{bib:Kim2007} & -0.02 (0.54, 10) & $\beta$-catenin/TCF complex\\
IL6 signaling \cite{bib:Singh2006} & -0.05 (0.69, 9) & nuclear STAT3\\
G1 cell cycle progression \cite{bib:Haberichter2007} & -0.57 (0.05, 9) & hypo- and hyper-phosphorylated Rb\\
Rho-kinase activation \cite{bib:Maeda2006} & -0.19 (0.28, 15) & phosphorylated myosin light chain\\
Arachidonic acid metabolism \cite{bib:Yang2007} & -0.57 (0.05, 10) & PGE2 and LTB4\\
TNF-driven apoptosis \cite{bib:Albeck2008} & -0.22 (0.34, 12) & the apoptosome\\
$\beta$-adrenergic signaling \cite{bib:Neves2008} & -0.18 (0.32, 9) & active MAP kinase\\
\hline
expected sign & $-$ \\
 total of expected sign & 12 \\
\end{tabular}
