# Supplementary material for: Proteins with greater influence on network dynamics evolve more slowly but are not more essential
Source: arXiv:0909.2889 source file (2009-09-20)
Supplement: Supplementary file 4 [file supp_mammals.tex]

\begin{tabular}{cc}
system & $r_{dN/dS,D}$ (p-val, N)\\
\hline
Insulin/EGF signaling \cite{bib:Borisov2009} & -0.28 (0.17, 13)\\
Heregulin/EGF signaling \cite{bib:Birtwistle2007} & -0.23 (0.21, 14)\\
NGF/EGF signaling (smaller) \cite{bib:Brown2004} & -0.58 (0.07, 8)\\
NGF/EGF signaling (larger) \cite{bib:Sasagawa2005} & -0.27 (0.15, 17)\\
EGF receptor endocytosis \cite{bib:Ung2008} & -0.03 (0.45, 25)\\
Wnt/ERK crosstalk \cite{bib:Kim2007} & -0.37 (0.14, 10)\\
IL6 signaling \cite{bib:Singh2006} & -0.30 (0.21, 10)\\
G1 cell cycle progression \cite{bib:Haberichter2007} & -0.31 (0.19, 10)\\
Rho-kinase activation \cite{bib:Maeda2006} & -0.10 (0.40, 16)\\
Arachidonic acid metabolism \cite{bib:Yang2007} & -0.49 (0.08, 10)\\
TNF-driven apoptosis \cite{bib:Albeck2008} & -0.11 (0.41, 12)\\
$\beta$-adrenergic signaling \cite{bib:Neves2008} & +0.70 (0.98, 9)\\
\hline
expected sign & $-$ \\
 total of expected sign & 11 \\
\end{tabular}
