# Supplementary material for: Proteins with greater influence on network dynamics evolve more slowly but are not more essential
Source: arXiv:0909.2889 source file (2009-09-20)
Supplement: Supplementary file 5 [file supp_unique.tex]

\begin{tabular}{cc}
system & $r_{dN/dS,D}$ (p-val, N)\\
\hline
Insulin/EGF signaling \cite{bib:Borisov2009} & -0.61 (0.08, 6)\\
Heregulin/EGF signaling \cite{bib:Birtwistle2007} & -0.63 (0.06, 6)\\
NGF/EGF signaling (smaller) \cite{bib:Brown2004} & --- (---, 1)\\
NGF/EGF signaling (larger) \cite{bib:Sasagawa2005} & -0.39 (0.21, 7)\\
EGF receptor endocytosis \cite{bib:Ung2008} & -0.01 (0.49, 10)\\
Wnt/ERK crosstalk \cite{bib:Kim2007} & -0.42 (0.16, 7)\\
IL6 signaling \cite{bib:Singh2006} & -0.28 (0.24, 10)\\
G1 cell cycle progression \cite{bib:Haberichter2007} & -0.31 (0.19, 10)\\
Rho-kinase activation \cite{bib:Maeda2006} & -0.26 (0.20, 14)\\
Arachidonic acid metabolism \cite{bib:Yang2007} & -0.53 (0.06, 10)\\
TNF-driven apoptosis \cite{bib:Albeck2008} & -0.14 (0.36, 12)\\
$\beta$-adrenergic signaling \cite{bib:Neves2008} & +0.26 (0.71, 7)\\
\hline
expected sign & $-$ \\
 total of expected sign & 10 \\
\end{tabular}
